# Supplementary material for: GSFF-SLAM: 3D Semantic Gaussian Splatting SLAM via Feature Field
Source: arXiv:2504.19409 source file (2025-05-16)
Supplement: Supplementary file 1 [file supplementary.tex]

\clearpage

\appendix
\section{Implementation Details}

\subsection{Hyperparameters}
In the following, we report the implementation details and hyperparameters used in our method to achieve high-precision tracking and mapping.

\noindent\textbf{Default Settings.} We set $N = 128$ to construct our feature field, where the learning rate for semantic features is 0.01, and optimization is performed using the Adam optimizer. We set $\lambda_t = 0.9$ and $\lambda_m = 0.9$ to balance the losses of RGB and depth images, and $\lambda_r = 10$ to balance the regularization loss, ensuring a uniform size of 3D Gaussians in the scene. The learning rates for other parameters of Gaussian points are shown in the \cref{tab:params_lr}.

\noindent\textbf{Tracking Settings.} We track the position of each frame, with a maximum optimization iteration of 200 per frame. The tracking optimization for the current frame terminates when the convergence threshold of $1\text{e-}4$ is reached. For the Replica dataset, we maintain a keyframe optimization window length of 5 to improve the effectiveness of re-tracking after subsequent map reconstruction. For the ScanNet dataset, we maintain a keyframe optimization window length of 4.

\noindent\textbf{Mapping Settings.} For the initial frame, we set the number of initialization iterations to 1000. For each subsequent keyframe, we set the number of optimization iterations to 20. For the Replica dataset, we maintain a mapping window length of 10, while for the ScanNet dataset, we maintain a mapping window length of 8.

\noindent\textbf{Semantic Mapping Settings.} Semantic mapping is always performed after appearance and geometric mapping. For the initial frame, we set the number of iterations to 10. For ground truth signals, since we use the cross-entropy function as the loss, the number of iterations for subsequent keyframes is set to 3.  For noisy textual signals, as we use the L1 loss and do not want excessive optimization in each frame that could lead to forgetting previously learned features, we set the number of iterations to 1. We align both the supervision signals and the re-rendered feature maps to a size of $\mathbb{R}^{480 \times 360 \times 512}$ to reduce memory usage while maintaining accuracy.

\begin{table}[t]
    \centering
    \begin{tabular}{lll}
    \toprule
                                     & Parameter Name            & Value     \\
    \midrule
    \multirow{8}{*}{\(\mathcal{G}\)} & position\_lr\_init        & 0.0008    \\
                                     & position\_lr\_final       & 0.0000016 \\
                                     & position\_lr\_delay\_mult & 0.01      \\
                                     & position\_lr\_max\_steps  & 30000     \\
                                     & color\_lr                 & 0.0025    \\
                                     & opacity\_lr               & 0.05      \\
                                     & scaling\_lr               & 0.005     \\
                                     & rotation\_lr              & 0.001     \\
    \hline
    \multirow{2}{*}{\(\delta\)}   & rotation\_delta\_lr       & 0.003     \\
                                     & trans\_delta\_lr          & 0.001    \\
    \bottomrule
    \end{tabular}
    \caption{Learning rate of main learnable parameters. For the position parameters, we use the exponential learning rate scheduler to adjust them.}
    \label{tab:params_lr}
\end{table}

\subsection{Flowchart}

As shown in \cref{fig:flowchart}, our system is divided into two threads: tracking and mapping. The semantic mapping is separated from the appearance and geometric mapping, allowing it to be flexibly enabled or disabled as needed. During tracking, we determine whether a frame is a keyframe. When a keyframe is detected, the mapping thread is activated. Instead of using a thread lock to wait for mapping to complete, we continue tracking the next frame. Once the background mapping thread finishes, it sends a request to update the parameters of the 3D Gaussians.

% 如图所示，我们的system分为tracking和mapping两个线程，其中semantic mapping与外观与几何的mapping分离，可以通过使能或失能灵活的添加和删除这个过程。我们在tracking过程中判断是否为关键帧，当检测到关键帧时激活建图线程，我们没有采用线程锁等待建图完成，而是继续追踪下一帧，当后台的建图线程完成后会发送请求进行3D Gaussians的参数更新。

\begin{figure}
    \centering
    \includegraphics[width=\linewidth]{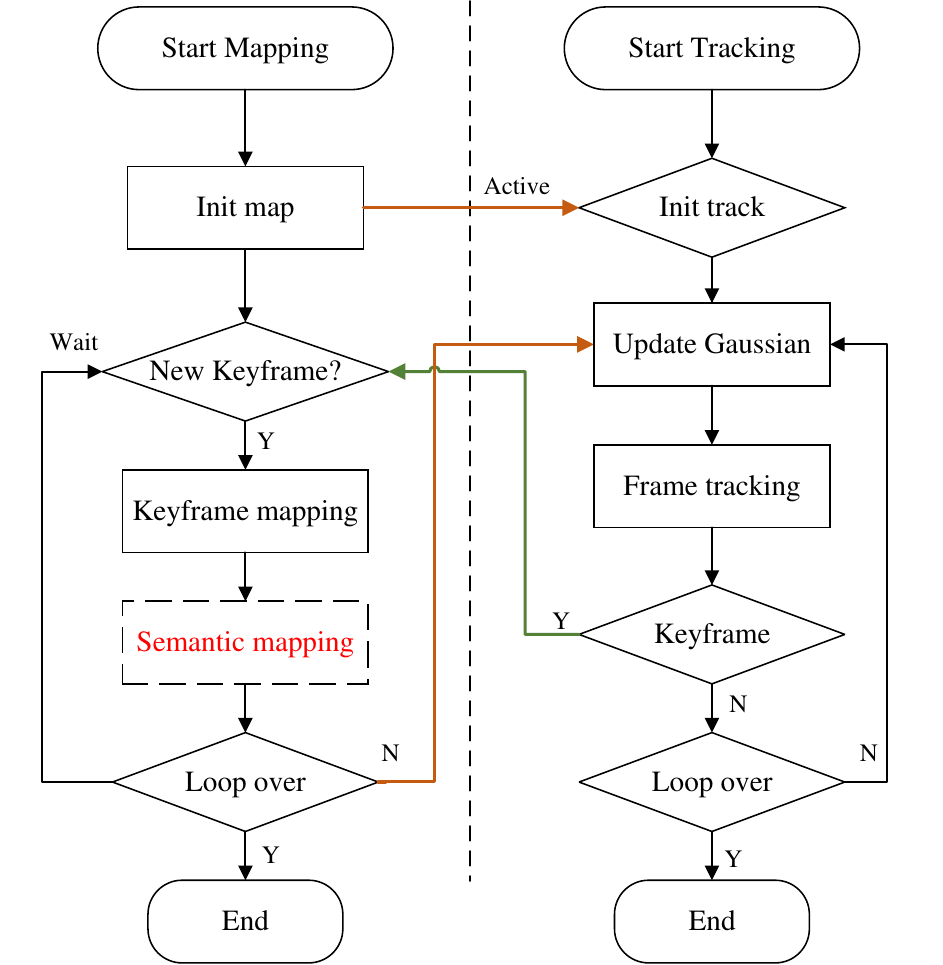}
    \caption{Our system is designed with a dual-threaded architecture, with semantic mapping as an independent module.}
    \label{fig:flowchart}
\end{figure}

\section{More Semantic Results}

\subsection{Catastrophic Forgetting of NeRF-based Method}

\begin{figure*}[!t]
   \centering
   \includegraphics[width=\linewidth]{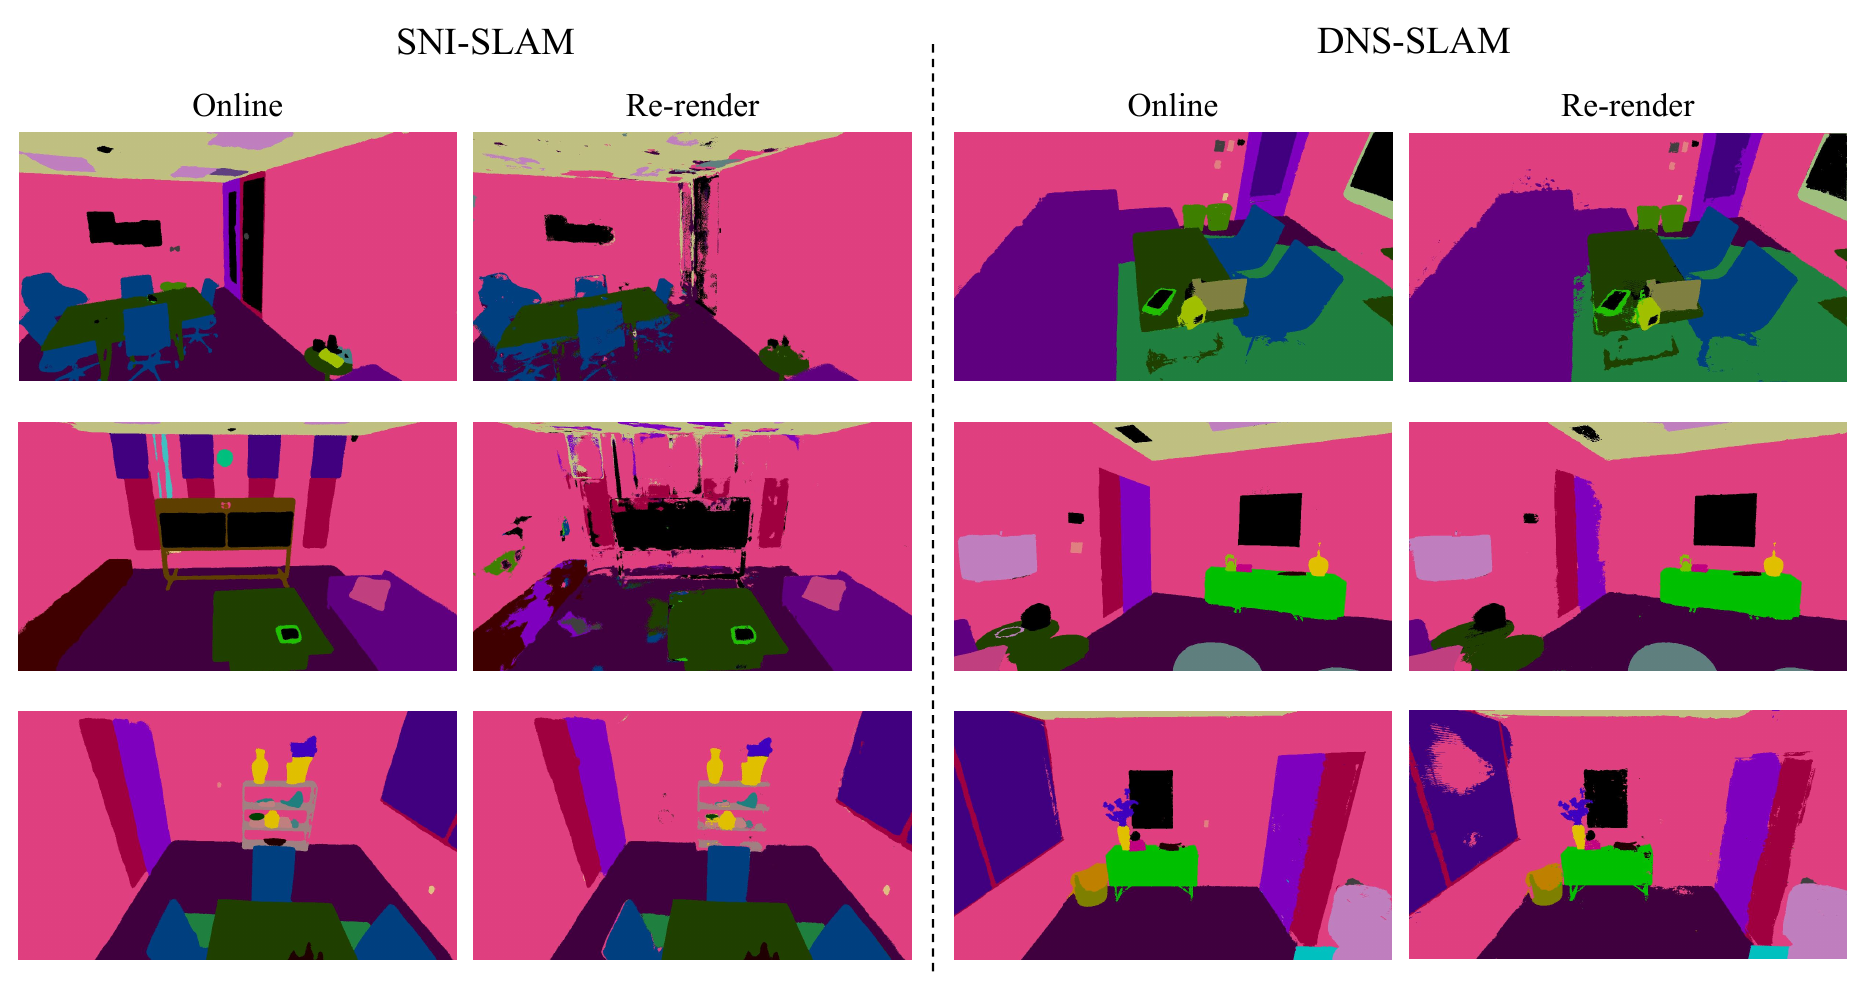}
   \caption{The NeRF-based baseline methods are significantly affected by catastrophic forgetting, as demonstrated by our experimental results on the Replica dataset.}
   \label{fig:NeRF_Shortcoming}
\end{figure*}

As shown in the \cref{fig:NeRF_Shortcoming}, we illustrate the catastrophic forgetting problem in SNI-SLAM and DNS-SLAM. Online represents the rendering result after completing semantic optimization for the current frame, while Rerender refers to the visualization result obtained by re-rendering after all frames have been processed (2000 frames for the Replica dataset). We present the most representative examples, where SNI-SLAM exhibits severe degradation, while DNS-SLAM also suffers from varying degrees of degradation. 
% This issue significantly impacts the application of Semantic SLAM methods in downstream tasks.

% 如图所示，我们展示了SNI-SLAM和DNS-SLAM的灾难性遗忘问题，其中Online表示的是其在完成当前帧的语义优化后，进行渲染的结果，rerender表示的是在完成所有帧（replica为2000帧）后，重新渲染得到的可视化结果。我们选取了最具代表性的几个样例进行展示，其中SNI-SLAM的退化问题较为严重，而DNS-SLAM也在不同程度上出现了退化。这个问题严重影响了Semantic SLAM方法在下游任务中的应用。

\begin{figure*}[t]
   \centering
   \includegraphics[width=\linewidth]{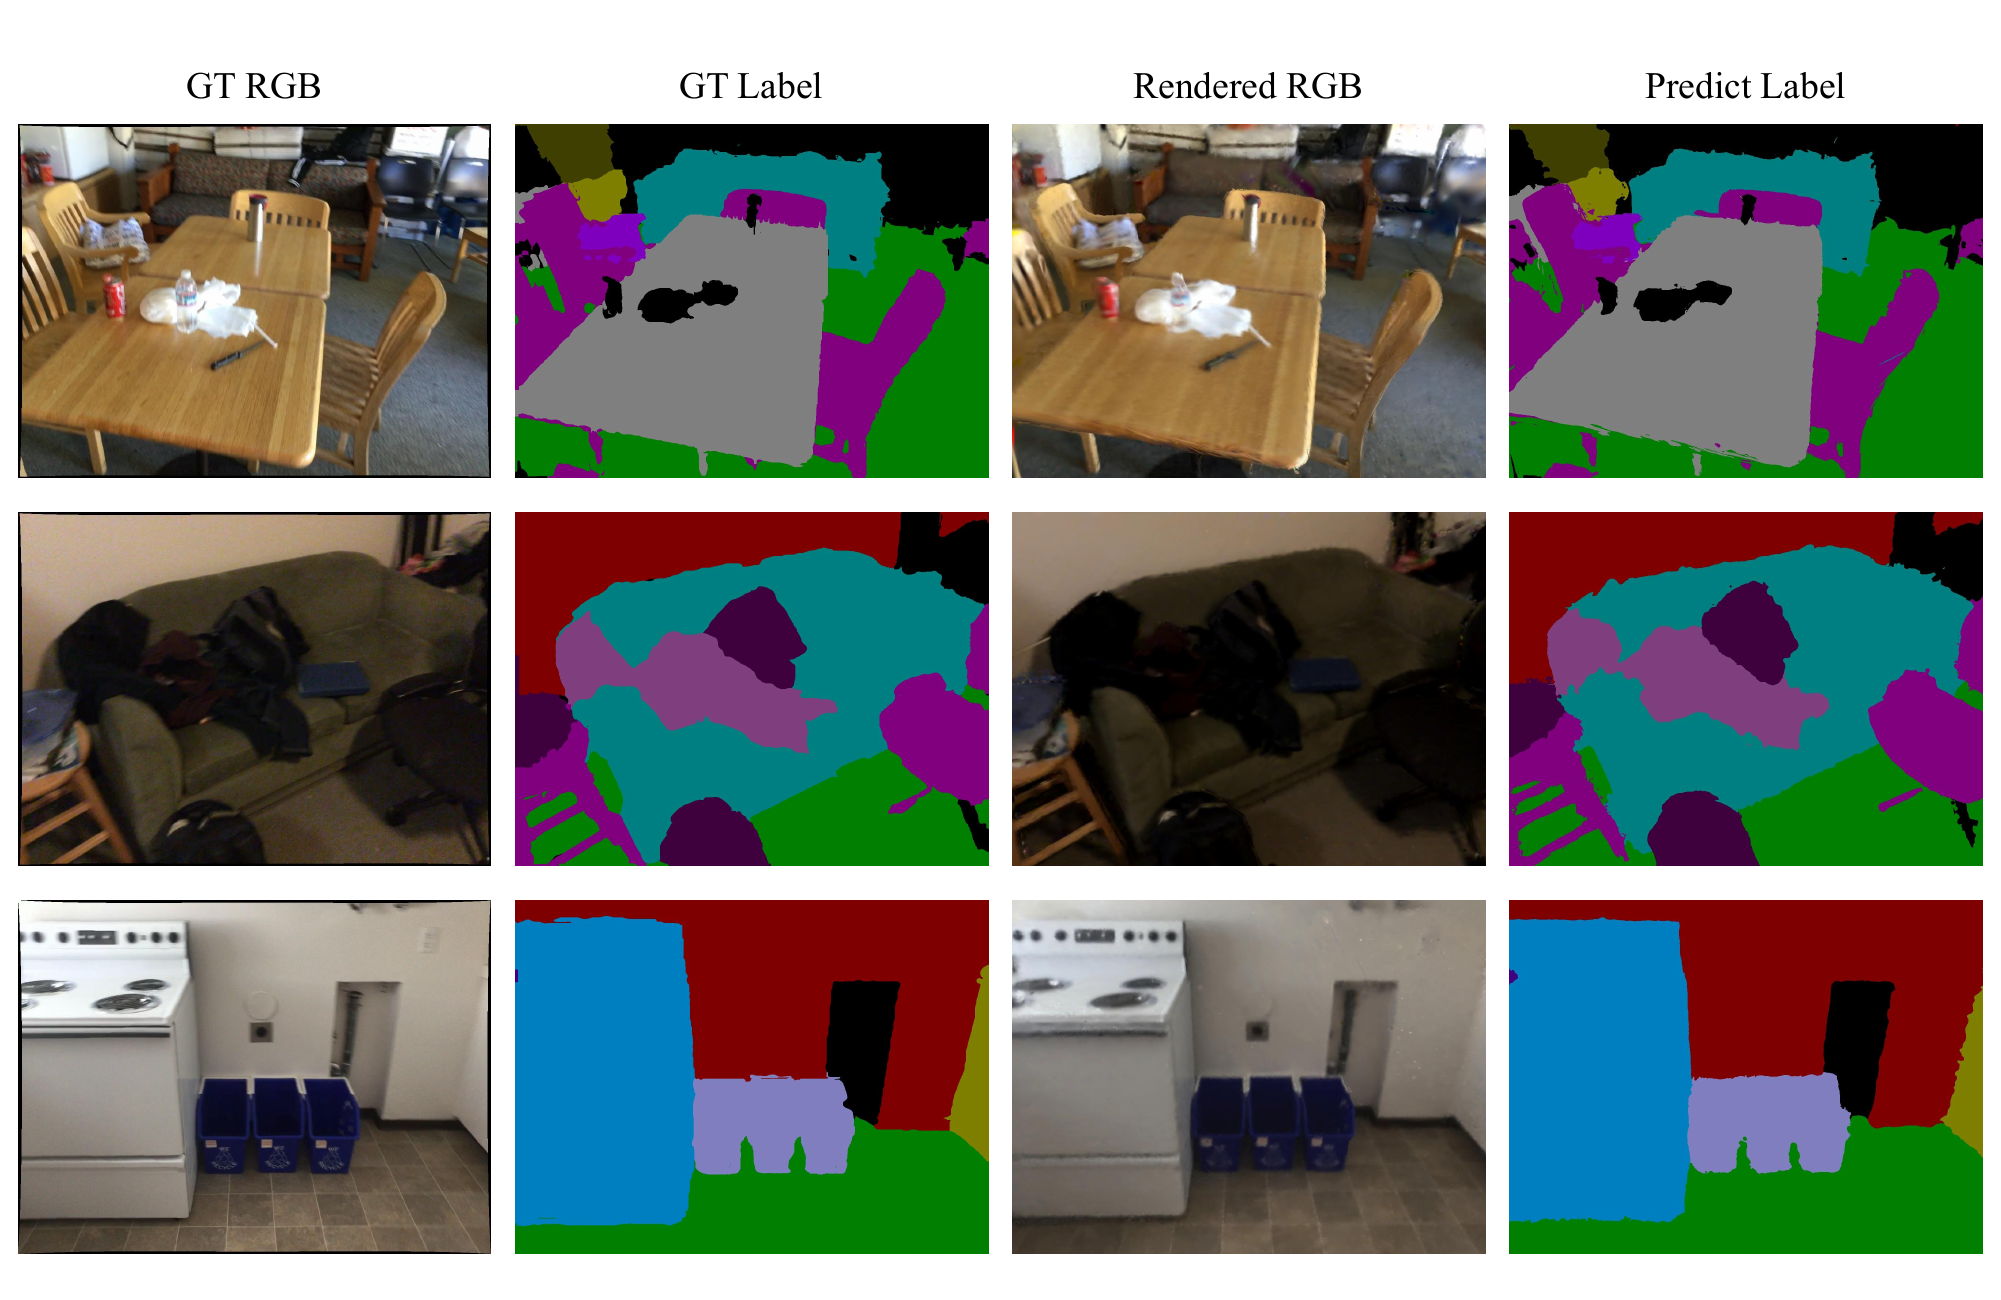}
   \caption{Rendering and semantic segmentation results on the ScanNet dataset.}
   \label{fig:vis_scannet}
\end{figure*}

\begin{figure*}[t]
   \centering
   \includegraphics[width=\linewidth]{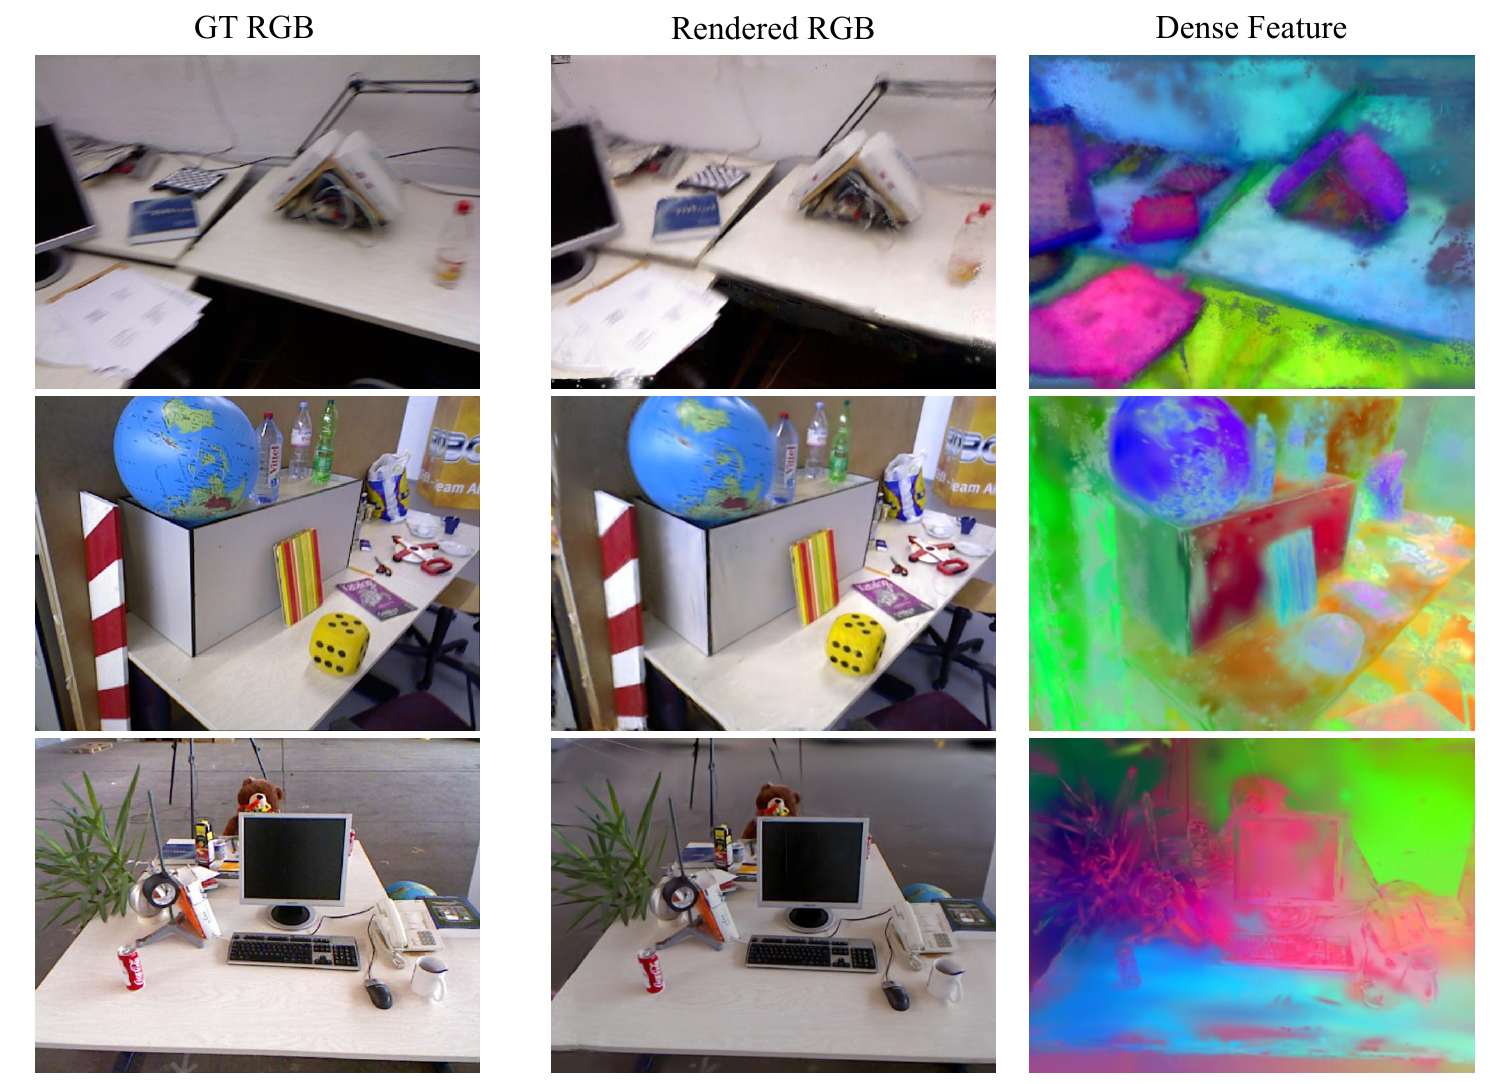}
   \caption{Rendering results on the TUM-RGBD dataset using patch-level feature and visualization results are obtained by PCA.}
   \label{fig:vis_tum}
\end{figure*}

\subsection{More visualization}

\noindent\textbf{ScanNet}. As illustrated in the \cref{fig:vis_scannet}, we present the rendering and semantic segmentation results on the ScanNet dataset. The semantic labels in ScanNet are not perfectly aligned with the RGB images and contain certain levels of annotation noise. Additionally, the scene images exhibit pixel noise, uneven lighting conditions, and motion blur, which lead to illumination loss and localized rendering artifacts in the synthesized views. These challenges highlight the difficulty of performing semantic SLAM on such a high-noise dataset.

\noindent\textbf{TUM-RGBD}. As shown in the \cref{fig:vis_tum}, we demonstrate the results of using feature maps from a ViT-based foundational model as 2D priors on the TUM-RGBD dataset. We render both the reconstructed RGB images and the dense feature maps. While the typical ViT paradigm produces sparse feature maps of size \( \mathbb{R}^{\frac{H}{16} \times \frac{W}{16} \times D} \), our rendering pipeline achieves dense feature maps of size \( \mathbb{R}^{H \times W \times D} \). Notably, the visualization of the feature maps reveals fine-grained local details.

% \textbf{ScanNet} 如图所示，我们展示了在ScanNet 数据集的渲染与语义分割结果，Scannet的语义标签没有和RGB图像完整对齐，并且存在一定的语义标注噪声，另外是场景图像存在像素噪声、不均匀的光照情况以及镜头运动模糊，这也导致了渲染图像存在一定的光照损失，和局部的渲染模糊现象。这也证明在这种高噪声数据集上进行语义SLAM的挑战性。

% \textbf{TUM-RGBD} 如图所示，我们展示了在TUM-RGBD数据集上采用ViT结构的基础模型的特征图作为2D先验的结果，我们渲染了重建的RGB图像和密集特征图。典型的ViT范式的基础模型产生R^{H/16, W/16，D}的稀疏特征图，我们的渲染管道可以实现R^{H, W，D}的密集特征图。值得注意的是特征图的可视化结果展现了较为细节的局部特征。

% \subsection{Comparative Experiment1: Sparse \& Noisy}

% \begin{figure*}[!t]
%    \centering
%    \includegraphics[width=\linewidth]{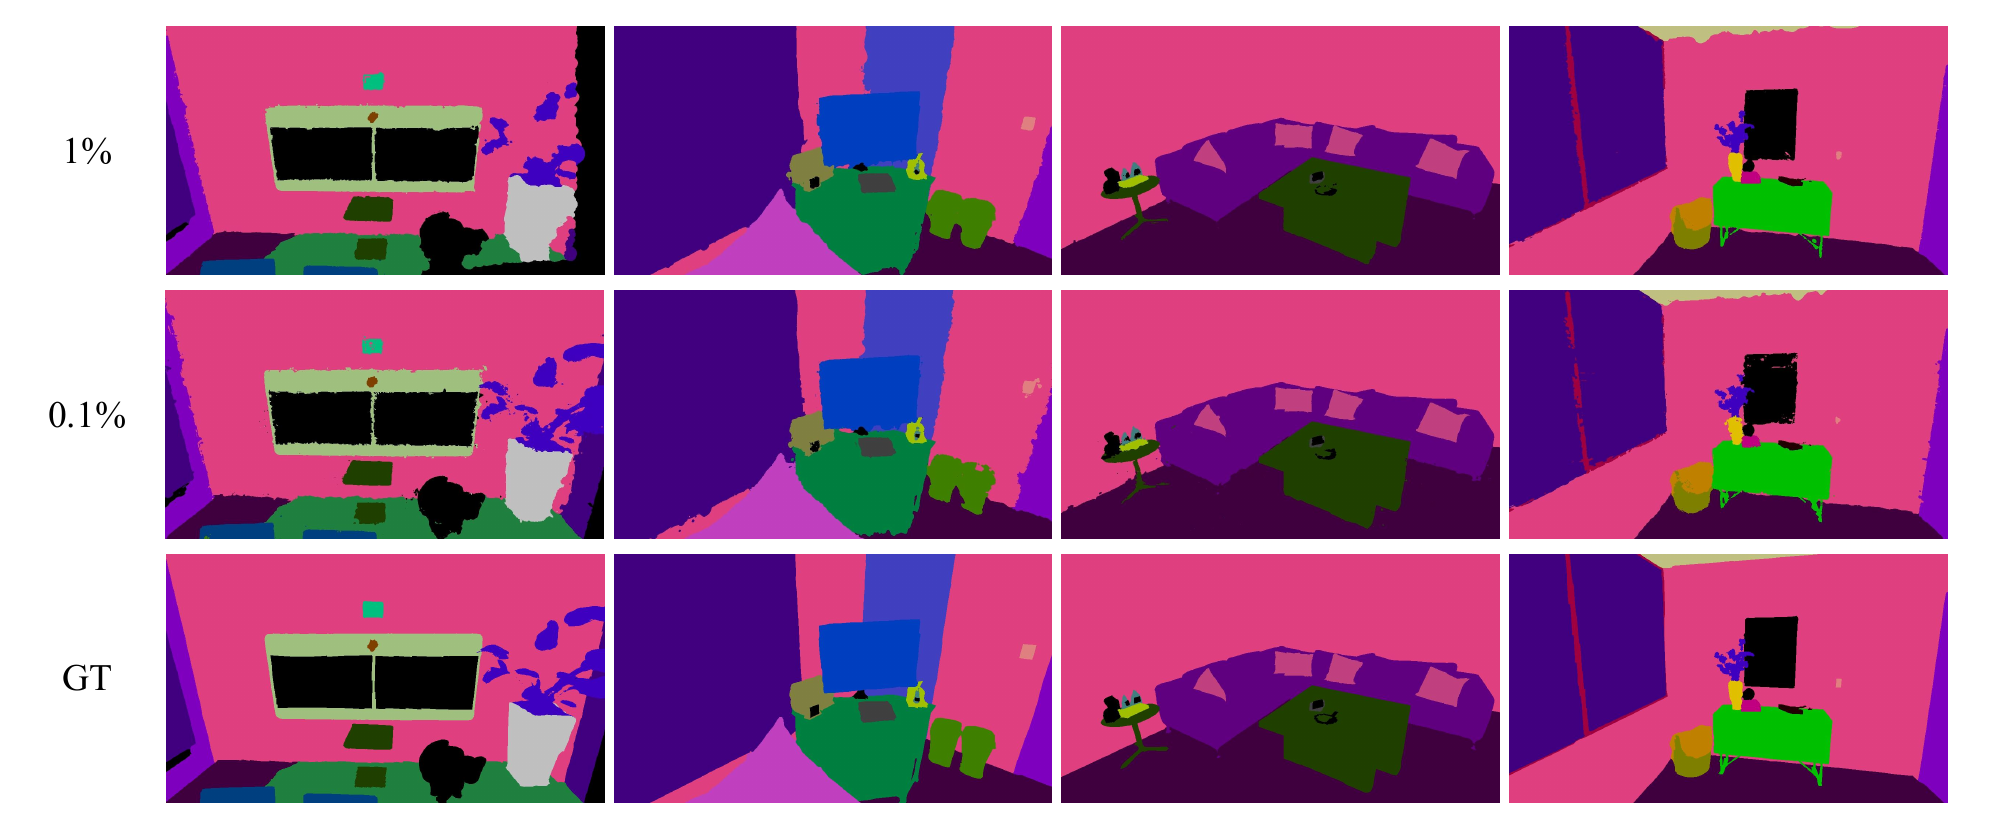}
%    \caption{Qualitative comparison on rendering quality of baseline and our method. }
%    \label{fig:sparse_gt}
% \end{figure*}

% \begin{figure*}[!t]
%    \centering
%    \includegraphics[width=\linewidth]{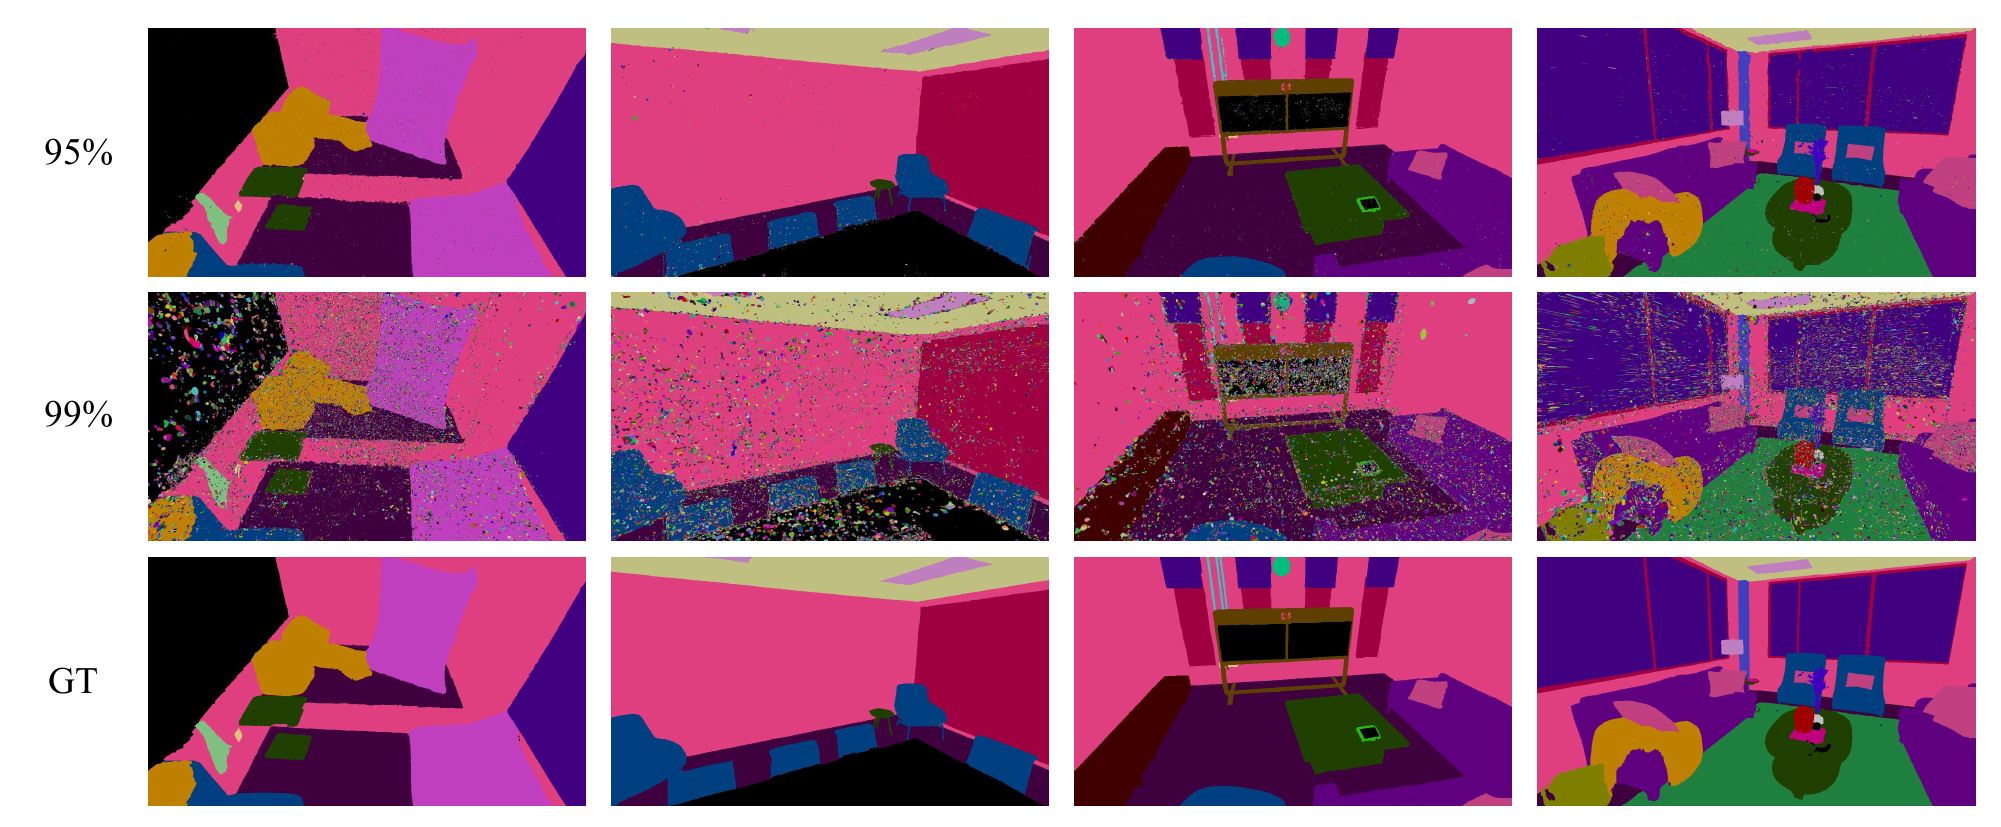}
%    \caption{Qualitative comparison on rendering quality of baseline and our method. }
%    \label{fig:noise_gt}
% \end{figure*}

% 如图所示是我们不断稀疏监督信号后其语义分割性能的变化，我们测试了稀疏信号对Semantic SLAM的影响，我们观察到即使采用0.1%的pixel-level的稀疏信号，仍然能重建出来较好的结果. 我们观察到一种现象“语义扩散”，具体的说，有信号的pixel会向周围像素扩散, 这使得稀疏的监督信号被致密化,这种现象导致了语义的边缘被损坏.
% 我们还展示了如图所示的密集噪声信号进行监督, 我们发现"语义扩散"现象同样影响到噪声信号的重建过程, 每个像素表现为临近像素的监督信号均值.由于采用了密集的信号,其在语义边缘的精确度并没有因此降低.
% 但是这两项实验仅在像素级别上进行了讨论,没有考虑到现实环境中存在的噪声往往是区域级的噪声以及还有个别物品存在稳定的识别错误. 这两项实验为我们前文中带噪声的稀疏先验监督提供了一定的作证.

% \begin{figure}[!t]
%    \centering
%    \includegraphics[width=0.9\linewidth]{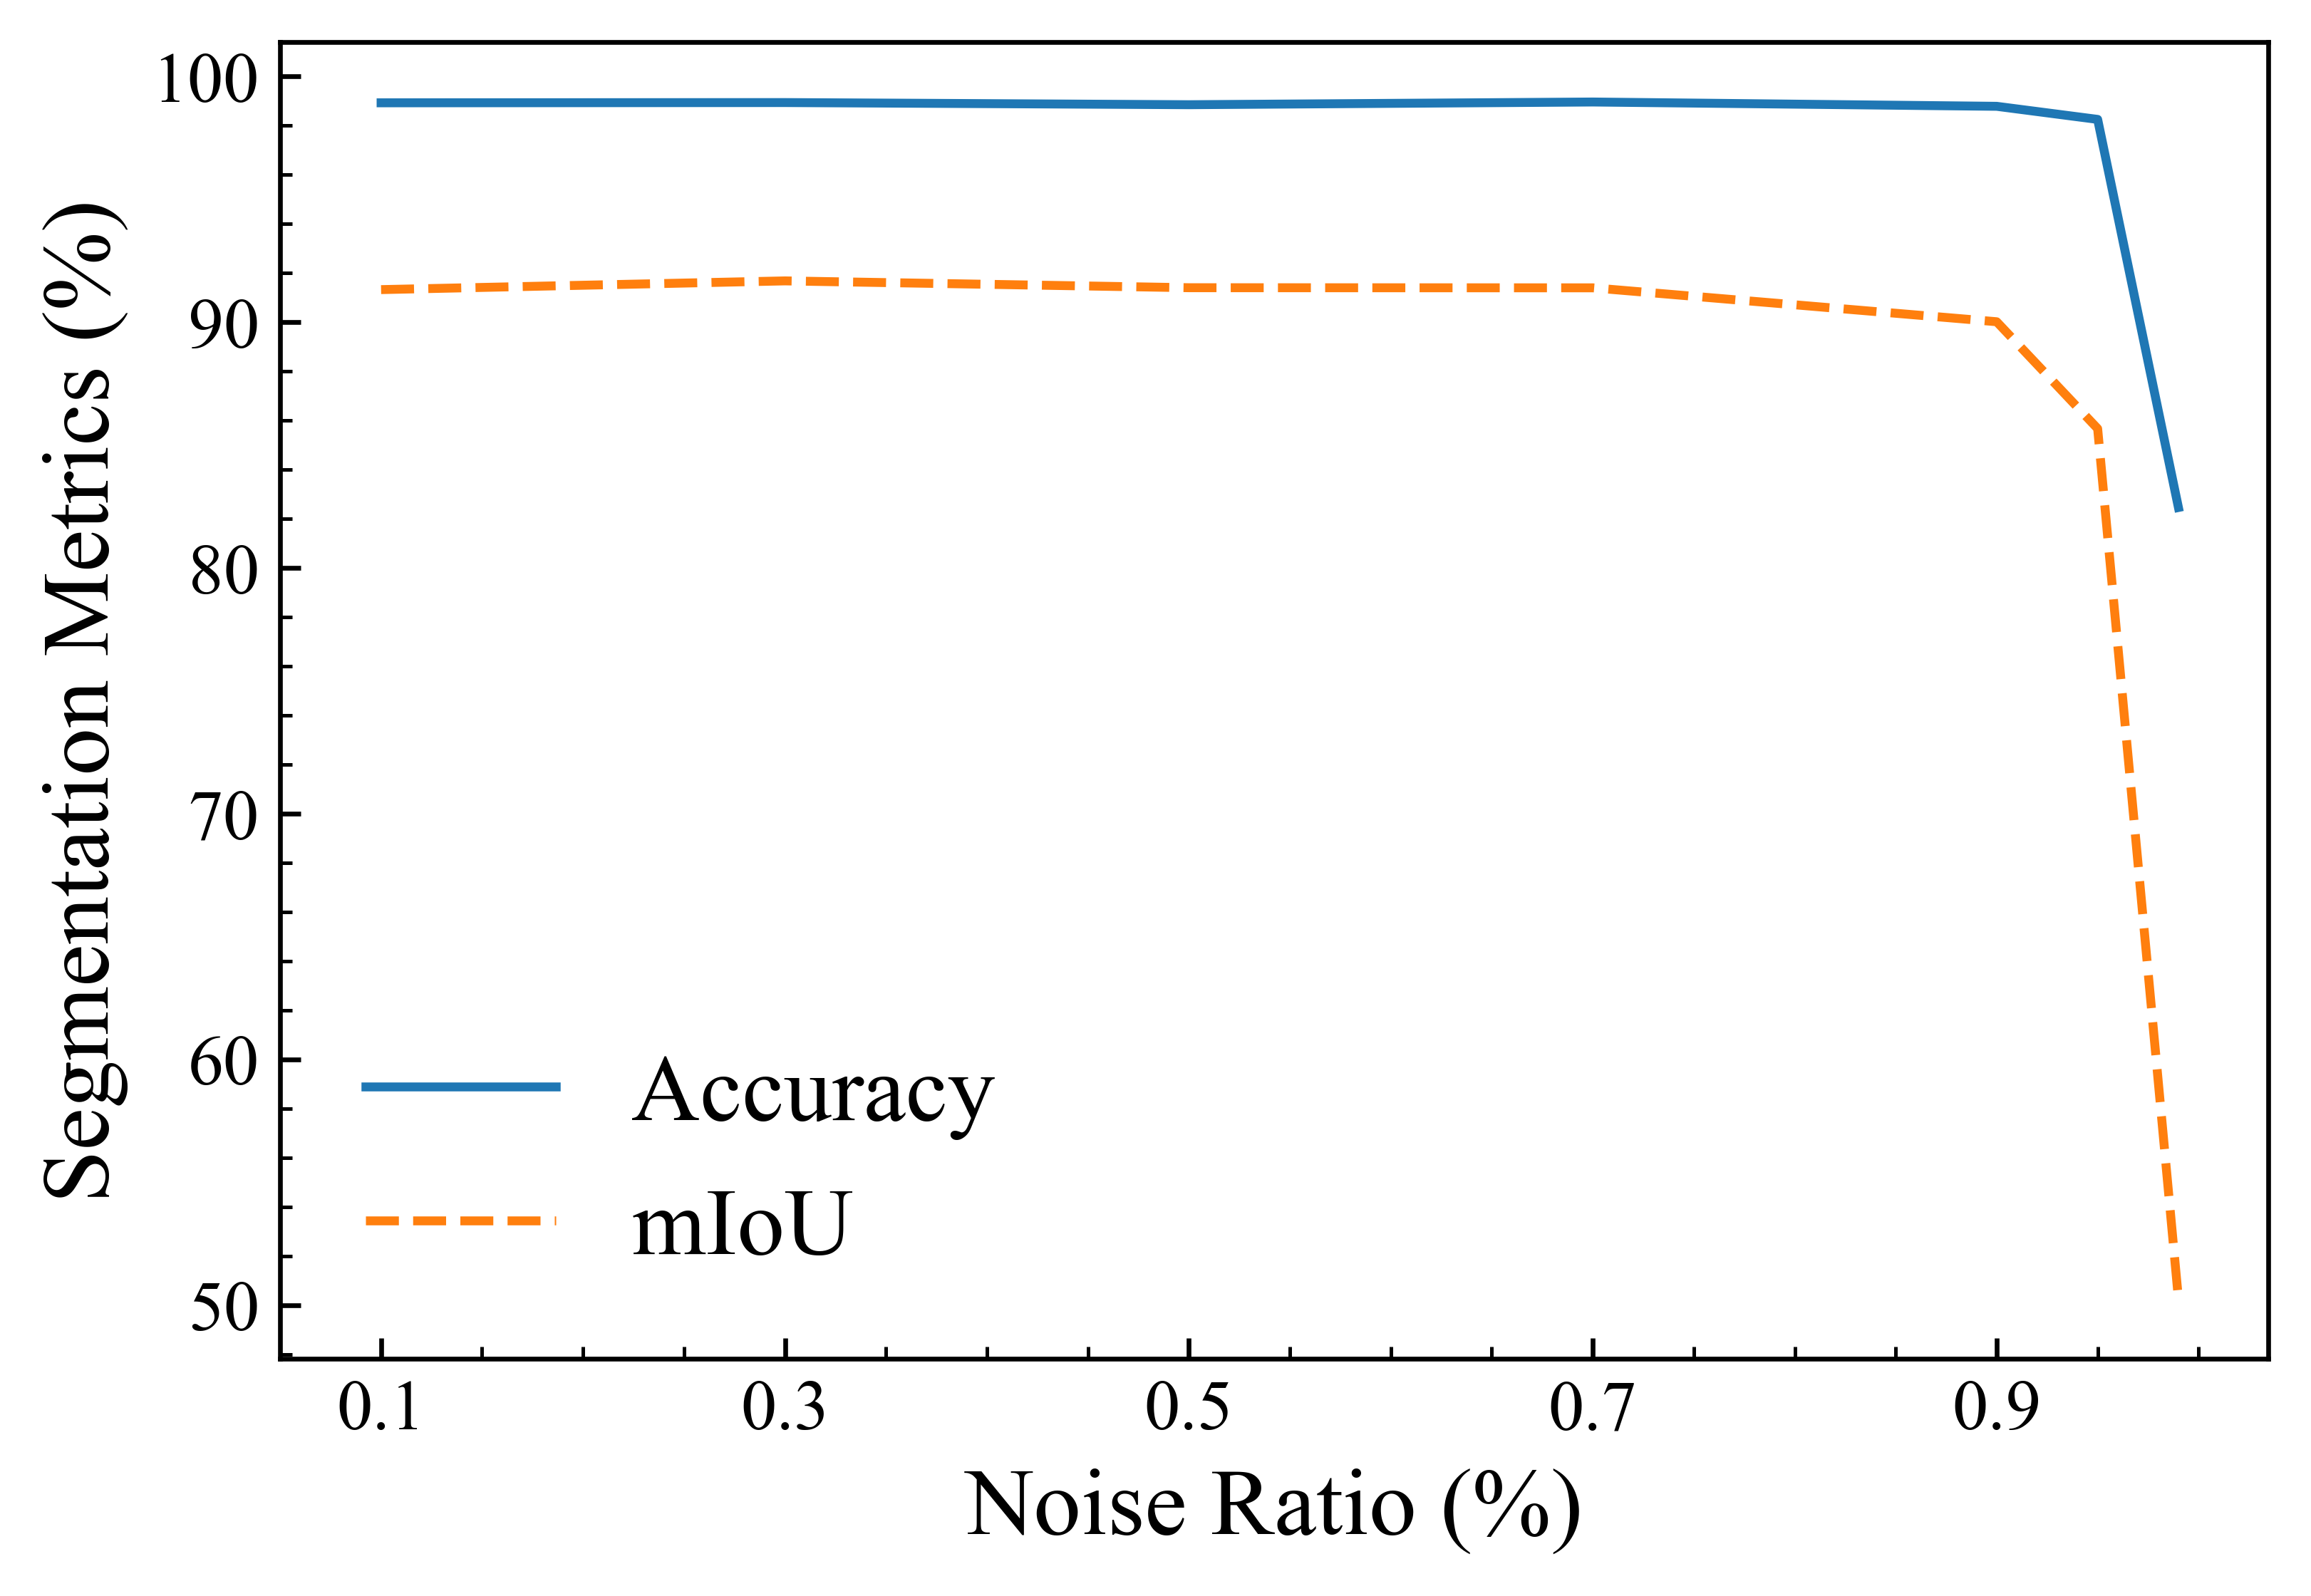}
%    \caption{Quantitative performance of GSFF-SLAM trained on Replica with pixel-level noise semantic labels. }
%    \label{fig:Noise GT}
% \end{figure}
